# Supplementary material for: A Unified Model for Non-Fickian Diffusion and Anomalous Swelling of Glassy Polymer Gels
Source: arXiv:2402.03844 ancillary file (2024-04-23)
Supplement: Supplementary file 1 [file SI.pdf]

# Supporting Information for
# A Unified Model for Non-Fickian Diffusion and Anomalous Swelling of Glassy Polymer Gels

Peihan Lyu,[1] Zhaoyu Ding,[1] Masao Doi,[1,2,*] and Xingkun Man[1,3,†]

[1] *School of Physics, Beihang University, Beijing 100191, China*

[2] *Wenzhou Institute, University of Chinese Academy of Sciences, Wenzhou 325000, China*

[3] *Peng Huanwu Collaborative Center for Research and Education, Beihang University, Beijing 100191, China*

[*] masao.doi@buaa.edu.cn

[†] manxk@buaa.edu.cn

In this Supplementary material, we show detailed derivation of our theoretical model, and explain how we numerically obtain the front velocity and the characteristic times.

## I. THEORETICAL MODEL

We consider a square sheet of glassy polymers that is initially homogenous and isotropic with thickness $2h_0$ and side length $L_0$ ($h_0 \ll L_0$). We take a Cartesian coordinate such that the left and right surfaces are at $z = \pm h_0$. The non-equilibrium state of such system is described by the displacement vector $\boldsymbol{u}(\boldsymbol{r}, t)$ which stands for the displacement of a point located at $\boldsymbol{r}$ in polymer network of dry state. We assume that the deformation is small, i.e., the strain $\varepsilon_{\alpha\beta} = \partial u_\alpha / \partial r_\beta \ll 1$ ($\alpha, \beta$ stand for $x, y, z$). The swelling of the polymer should be uniform and isotropic in the lateral $x$-$y$ plane due to the thin disk geometry of the sample ($L_0 \gg h_0$). Moreover, the system has the symmetry with respect to the middle plane at $z = 0$ because solvents permeate into the sample from both surfaces at $z = \pm h_0$ simultaneously. We assume that the displacement in the $x$, $y$ and $z$-directions are

$$u_x = \alpha(t)x \tag{1}$$

$$u_y = \alpha(t)y \tag{2}$$

$$u_z = u(z, t) \tag{3}$$

where $\alpha(t)$ is the strain in the $x$-$y$ plane, $u(z, t)$ is the displacement normal to the surface. This leads to the fact that the strain tensor only has diagonal component, which is

$$\varepsilon_x = \frac{\partial u_x}{\partial x} = \alpha(t) \tag{4}$$

$$\varepsilon_y = \frac{\partial u_y}{\partial y} = \alpha(t) \tag{5}$$

$$\varepsilon_z = \frac{\partial u_z}{\partial z} = \frac{\partial u(z, t)}{\partial z} \tag{6}$$

We assume that both polymer and solvent are incompressible, i.e., $\phi_s(\boldsymbol{r}, t) + \phi_p(\boldsymbol{r}, t) = 1$. Here $\phi_p(\boldsymbol{r}, t)$ and $\phi_s(\boldsymbol{r}, t)$ are volume fraction of polymer and solvent, respectively. In the present problem, we always take the dry state (no solvent) of the sample as the reference state. Then, the volume fraction of the polymer $\phi_p$ can be calculated from $\boldsymbol{u}(\boldsymbol{r}, t)$ by

$$\phi_p(\boldsymbol{r}, t) = \frac{1}{\det[\nabla(\boldsymbol{r} + \boldsymbol{u})]} \tag{7}$$

In our system, eqs. (1), (2) and (3) give that

$$\phi_p(\boldsymbol{r},t) = \frac{1}{(1+\alpha)^2(1+\frac{\partial u}{\partial z})} \approx 1 - 2\alpha - \frac{\partial u}{\partial z} \tag{8}$$

and

$$\phi_s(\boldsymbol{r},t) \approx \frac{\partial u}{\partial z} + 2\alpha = \nabla \cdot \boldsymbol{u} \tag{9}$$

The velocity $\boldsymbol{v}_p(\boldsymbol{r})$ of polymer at $\boldsymbol{r}$ is given by the partial derivative of $\boldsymbol{u}(\boldsymbol{r},t)$ with respect to time, i.e., $\boldsymbol{v}_p = \dot{\boldsymbol{u}}$. The polymer velocity $\boldsymbol{v}_p$ is generally different from solvent velocity $\boldsymbol{v}_s$. However, $\boldsymbol{v}_p$ and $\boldsymbol{v}_s$ cannot be independent since they have to satisfy the incompressibility condition. As the system is imcompressible, we have

$$\nabla \cdot (\phi_p \boldsymbol{v}_p + \phi_s \boldsymbol{v}_s) = 0 \tag{10}$$

As we are considering a thin film with $L_0 \gg h_0$, the relative motion in the $x$-$y$ direction causes huge amount of energy dissipation. We may assume that $v_{\rm sx} = v_{\rm px}$, $v_{\rm sy} = v_{\rm py}$ and the relative motion takes place only in the z-direction. Then eq. (10) becomes

$$2\dot{\alpha} + \frac{\partial}{\partial z}(\phi_p \dot{u} + \phi_s v_{\rm sz}) = 0 \tag{11}$$

Notice that the symmetry with respect to the midplane at $z = 0$ gives boundary conditions $u|_{z=0} = 0$ and $v_{\rm sz}|_{z=0} = 0$. Then, $v_{\rm sz}$ can be solved from eq. (11) as

$$v_{\rm sz} = \frac{-2\dot{\alpha} z - \phi_p \dot{u}}{\phi_s} \tag{12}$$

Therefore, the state of the sample at time $t$ is completely characterized by $u(z,t)$ and $\alpha(t)$.

To determine the time evolution of $u(z,t)$ and $\alpha(t)$, we use Onsager principle [1–3]. This principle states that the time evolution of non-equilibrium state specified by a set of state variables $(x_1, x_2, ...)$ is determined by the minimum condition of the Rayleighian $\Re$ with respect to the evolution rate $(\dot{x}_1, \dot{x}_2, ...)$. The Rayleighian $\Re$ is generally written as

$$\Re = \Phi + \dot{F} \tag{13}$$

where $\Phi$ is the dissipation function which represents the entropy production rate when the state variables are changing at rate $(\dot{x}_1, \dot{x}_2, ...)$, and $\dot{F}$ is the change rate of free energy $F$ which is defined by $\dot{F} = \sum_i \frac{\delta F}{\delta x_i} \dot{x}_i$.

## A. Free Energy

We use $\alpha(t)$ and $u(z,t)$ as the state variables for the swelling of glassy polymers. The free energy of glassy polymers is the same as it of soft polymers. The free energy density $f$ includes the elastic energy of the polymer network $f_{\rm ela}$ and the mixing energy of polymer and solvent $f_{\rm mix}$.

For small deformation, the elastic energy density is generally written as [4]

$$f_{\rm ela} = \frac{K}{2}(\sum_{\alpha} \varepsilon_{\alpha\alpha})^2 + \frac{G}{4}\sum_{\alpha\beta}\left(\varepsilon_{\alpha\beta} + \varepsilon_{\beta\alpha} - \frac{2}{3}\delta_{\alpha\beta}\sum_{\gamma}\varepsilon_{\gamma\gamma}\right)^2 \tag{14}$$

where $K$ and $G$ are material constants called osmotic bulk modulus and shear modulus respectively, and $\varepsilon_{\alpha\beta} = \partial u_\alpha/\partial r_\beta$ ($\alpha, \beta$ stand for $x, y, z$) are strains. Notice that here $K$ is the osmotic bulk modulus, rather than the bulk modulus. The osmotic bulk modulus $K$ is usually of the same order as the shear modulus $G$. This is because that when the polymer sheet is placed in a bath of solvent, the swollen of the sample is mainly induced by the solvent penetration, rather than the polymer itself. Therefore, the osmotic bulk modulus $K$ corresponding to polymer swelling induced by solvent penetration is much smaller than the bulk modulus for volume increasing of polymer itself. For the current problem, inserting expressions for strains in eqs. (4), (5) and (6) into eq. (14), we have

$$f_{\rm ela} = \frac{K}{2}\left(\varepsilon_x + \varepsilon_y + \varepsilon_z\right)^2 + \frac{G}{3}\left[(\varepsilon_x - \varepsilon_y)^2 + (\varepsilon_y - \varepsilon_z)^2 + (\varepsilon_z - \varepsilon_x)^2\right] \tag{15}$$

The mixing free energy $f_{\rm mix}$ is a function of $\phi_p$. According to the definition of the polymer volume fraction eq. (7) and the fact that only the diagonal components of the strain tensors are non-zero, we have

$$\begin{aligned}\phi_p &= \frac{1}{1+\varepsilon_x}\frac{1}{1+\varepsilon_y}\frac{1}{1+\varepsilon_z} \\ &\approx 1 - \varepsilon_x - \varepsilon_y - \varepsilon_z \end{aligned} \tag{16}$$

At the equilibrium state, we assume that all strains relax to an equilibrium strain $\varepsilon_{\rm eq}$, resulting in that the polymer volume fraction has an equilibrium value $\phi_p^{\rm eq} = 1 - 3\varepsilon_{\rm eq}$. Then, the total free energy density, $f = f_{\rm ela} + f_{\rm mix}$, at the equilibrium becomes $f_{\rm eq} = \frac{9}{2}K\varepsilon_{\rm eq}^2 + f_{\rm mix}(\phi_p^{\rm eq})$. The equilibrium state should have minimum free energy ($\partial f_{\rm eq}/\partial\varepsilon_{\rm eq} = 0$), which gives the condition for the equilibrium strain

$$9K\varepsilon_{\rm eq} - 3\left.\frac{\partial f_{\rm mix}}{\partial\phi_p}\right|_{\phi_p^{\rm eq}} = 0 \tag{17}$$

Since the deformation is small ($\varepsilon_\alpha \ll 1$), we can expand the free energy around the equilibrium strain,

$$f = f_{\text{eq}} + \sum_\alpha \left.\frac{\partial f}{\partial \varepsilon_\alpha}\right|_{\text{eq}} (\varepsilon_\alpha - \varepsilon_{\text{eq}}) + \frac{1}{2}\sum_{\alpha\beta} \left.\frac{\partial^2 f}{\partial \varepsilon_\alpha \varepsilon_\beta}\right|_{\text{eq}} (\varepsilon_\alpha - \varepsilon_{\text{eq}})(\varepsilon_\beta - \varepsilon_{\text{eq}}) + o\left[(\varepsilon - \varepsilon_{\text{eq}})^2\right] \quad (18)$$

where the first derivations are

$$\frac{\partial f}{\partial \varepsilon_x} = K(\varepsilon_x + \varepsilon_y + \varepsilon_z) + \frac{2}{3}G\left[(\varepsilon_x - \varepsilon_y) + (\varepsilon_x - \varepsilon_z)\right] - \frac{\partial f_{\text{mix}}}{\partial \phi_p} \quad (19)$$

$$\frac{\partial f}{\partial \varepsilon_y} = K(\varepsilon_x + \varepsilon_y + \varepsilon_z) + \frac{2}{3}G\left[(\varepsilon_y - \varepsilon_z) + (\varepsilon_y - \varepsilon_x)\right] - \frac{\partial f_{\text{mix}}}{\partial \phi_p} \quad (20)$$

$$\frac{\partial f}{\partial \varepsilon_z} = K(\varepsilon_x + \varepsilon_y + \varepsilon_z) + \frac{2}{3}G\left[(\varepsilon_z - \varepsilon_y) + (\varepsilon_z - \varepsilon_x)\right] - \frac{\partial f_{\text{mix}}}{\partial \phi_p} \quad (21)$$

As $\varepsilon_x = \varepsilon_y = \varepsilon_z = \varepsilon_{\text{eq}}$ at equilibrium state, eqns. (19)-(21) becomes zero according to the condition of eq. (17).

The second derivations at equilibrium state are

$$\frac{\partial^2 f}{\partial \varepsilon_x^2} = \frac{\partial^2 f}{\partial \varepsilon_y^2} = \frac{\partial^2 f}{\partial \varepsilon_z^2} = K + \frac{4}{3}G + \left.\frac{\partial^2 f_{\text{mix}}}{\partial \phi_p^2}\right|_{\phi_p^{\text{eq}}} \quad (22)$$

$$\frac{\partial^2 f}{\partial \varepsilon_x \partial \varepsilon_y} = \frac{\partial^2 f}{\partial \varepsilon_x \partial \varepsilon_z} = \frac{\partial^2 f}{\partial \varepsilon_y \partial \varepsilon_z} = K - \frac{2}{3}G + \left.\frac{\partial^2 f_{\text{mix}}}{\partial \phi_p^2}\right|_{\phi_p^{\text{eq}}} \quad (23)$$

Then, the free energy eq. (18) finally becomes

$$\begin{aligned} f - f_{\text{eq}} &= \frac{1}{2}\frac{\partial^2 f}{\partial \varepsilon_x^2}\left[(\varepsilon_x - \varepsilon_{\text{eq}})^2 + (\varepsilon_y - \varepsilon_{\text{eq}})^2 + (\varepsilon_z - \varepsilon_{\text{eq}})^2\right] \\ &\quad + \frac{\partial^2 f}{\partial \varepsilon_x \partial \varepsilon_y}\left[(\varepsilon_x - \varepsilon_{\text{eq}})(\varepsilon_y - \varepsilon_{\text{eq}}) + (\varepsilon_y - \varepsilon_{\text{eq}})(\varepsilon_z - \varepsilon_{\text{eq}}) + (\varepsilon_z - \varepsilon_{\text{eq}})(\varepsilon_x - \varepsilon_{\text{eq}})\right] \\ &= \frac{1}{2}\tilde{K}\left(\varepsilon_x + \varepsilon_y + \varepsilon_z - 3\varepsilon_{\text{eq}}\right)^2 + \frac{1}{3}G\left[(\varepsilon_x - \varepsilon_y)^2 + (\varepsilon_y - \varepsilon_z)^2 + (\varepsilon_z - \varepsilon_x)^2\right] \end{aligned} \quad (24)$$

where $\tilde{K} = K + \left.\frac{\partial^2 f_{\text{mix}}}{\partial \phi_p^2}\right|_{\phi_p^{\text{eq}}}$. Comparing with the elastic energy eq. (15), the mixing energy shifts the minimum point of the energy from $\varepsilon_x = \varepsilon_y = \varepsilon_z = 0$ to $\varepsilon_{\text{eq}}$, and gives a correction term to the osmotic bulk modulus $K$. We neglected the constant $f_{\text{eq}}$ and omitted the tilde mark on $K$ in main text. The total free energy of the current problem is

$$F = \int \mathrm{d}\boldsymbol{r}\, \frac{K}{2}\left(\varepsilon_x + \varepsilon_y + \varepsilon_z - 3\varepsilon_{\text{eq}}\right)^2 + \frac{G}{3}\left[(\varepsilon_x - \varepsilon_y)^2 + (\varepsilon_y - \varepsilon_z)^2 + (\varepsilon_z - \varepsilon_x)^2\right] \quad (25)$$

Inserting the expressions of the three strains into the free energy, we have

$$\frac{F}{L_0^2} = \int_{-h_0}^{h_0} \mathrm{d}z\, \left[\frac{K}{2}\left(2\alpha + \frac{\partial u}{\partial z} - 3\varepsilon_{\text{eq}}\right)^2 + \frac{2G}{3}\left(\frac{\partial u}{\partial z} - \alpha\right)^2\right] \quad (26)$$

## B. Dissipation Function

Having shown the free energy, we now turn to the dissipation function. The dissipation function $\Phi$ includes the friction dissipation between polymer and solvent $\Phi_{\rm dif}$, and the viscosity dissipation of polymer $\Phi_{\rm rhe}$. The friction dissipation is the same as that for soft gels in previous works [5–7], which is

$$\Phi_{\rm dif} = \int {\rm d}\boldsymbol{r} \frac{1}{2}\xi_0 (\boldsymbol{v}_p - \boldsymbol{v}_s)^2 \tag{27}$$

where $\xi_0$ is the friction coefficient per unit volume between polymer network and solvent. Using $v_{\rm px} = v_{\rm sx}$, $v_{\rm py} = v_{\rm sy}$, $v_{\rm pz} = \dot{u}$ and eq. (12) for $v_{\rm sz}$, $\Phi_{\rm dif}$ can be written as

$$\frac{\Phi_{\rm dif}}{L_0^2} = \int_{-h_0}^{h_0} {\rm d}z \frac{1}{2}\xi \left(\dot{u} + 2\dot{\alpha} z\right)^2 \tag{28}$$

Here we write $\xi = \xi_0/\phi_s^2$ as effective friction coefficient.

The viscosity dissipation is due to the viscosity of the polymer $\eta$, which is obtained by symmetry consideration, and can be written as

$$\Phi_{\rm rhe} = \int {\rm d}\boldsymbol{r} \frac{\eta}{4} \sum_{\alpha\beta} \left( \dot{\varepsilon}_{\alpha\beta} + \dot{\varepsilon}_{\beta\alpha} - \frac{2}{3}\delta_{\alpha\beta} \sum_{\gamma} \dot{\varepsilon}_{\gamma\gamma} \right)^2 \tag{29}$$

Here, $\eta$ is defined by $\eta = G\tau_{\rm rhe}$, where $\tau_{\rm rhe}$ is the rheological relaxation time. In literatures, $\eta$ is often called internal viscosity, and stands for the energy dissipation associated with the configurational change of polymer. If the deformation takes place satisfying the incompressible condition $\sum_\alpha \dot{\varepsilon}_{\alpha\alpha} = 0$, $\Phi_{\rm rhe}$ reduces to

$$\Phi_{\rm rhe} = \int {\rm d}\boldsymbol{r} \frac{\eta}{4} \sum_{\alpha\beta} \left( \dot{\varepsilon}_{\alpha\beta} + \dot{\varepsilon}_{\beta\alpha} \right)^2 \tag{30}$$

which is the energy dissipation function of viscous fluid [2].

Moreover, we can show that the material described by the Rayleighian $\Re = \Phi_{\rm rhe} + \dot{F}$ corresponds to the three-dimensional Kelvin-Voigt model. To derive the general constitutive relation, we take a free energy that only has the elastic energy, eq. (14). Then, the Rayleighian function becomes

$$\Re = \int {\rm d}\boldsymbol{r} \sum_{\alpha\beta} \left[ \frac{\partial f_{\rm ela}}{\partial \varepsilon_{\alpha\beta}} \dot{\varepsilon}_{\alpha\beta} + \frac{\eta}{4} \left( \dot{\varepsilon}_{\alpha\beta} + \dot{\varepsilon}_{\beta\alpha} - \frac{2}{3}\delta_{\alpha\beta} \sum_{\gamma} \dot{\varepsilon}_{\gamma\gamma} \right)^2 \right] \tag{31}$$

We define the density of Rayleighian function $R(\boldsymbol{r})$ so that $\Re = \int \mathrm{d}\boldsymbol{r} R(\boldsymbol{r})$, the stress is simply given by $\sigma_{ab} = \frac{\partial R}{\partial \dot{\varepsilon}_{ab}}$ ($a, b$ stand for $x, y, z$) [2], giving that

$$\begin{aligned}\sigma_{ab} =&\delta_{ab}\left[(K-\frac{2}{3}G)\sum_{\gamma}\varepsilon_{\gamma\gamma}-\frac{2}{3}\eta\sum_{\gamma}\dot{\varepsilon}_{\gamma\gamma}\right]+G(\varepsilon_{ab}+\varepsilon_{ba})+\eta(\dot{\varepsilon}_{ab}+\dot{\varepsilon}_{ba})\\ =&\delta_{ab}\lambda\left[\sum_{\gamma}\tilde{\varepsilon}_{\gamma\gamma}-\frac{2\eta}{3\lambda}\sum_{\gamma}\dot{\tilde{\varepsilon}}_{\gamma\gamma}\right]+2\mu\left[\tilde{\varepsilon}_{ab}+\tau_{\mathrm{rhe}}\dot{\tilde{\varepsilon}}_{ab}\right] \end{aligned}\tag{32}$$

Here $\tilde{\varepsilon}_{ab} = \frac{1}{2}(\varepsilon_{ab} + \varepsilon_{ba})$ is symmetric strain tensor, $\lambda = K - \frac{2}{3}G$ and $\mu = G$ are Lamé constants, $\tau_{\mathrm{rhe}} = \eta/G$ is rheological relaxation time. Equation (32) is just the constitutive relation of three-dimensional Kelvin-Voigt model [8].

In our system, inserting expressions for strains into eq. (31), the viscosity dissipation function can be written as

$$\frac{\Phi_{\mathrm{rhe}}}{L_0^2} = \int_{-h_0}^{h_0} \mathrm{d}z \frac{2}{3}\eta\left(\frac{\partial \dot{u}}{\partial z} - \dot{\alpha}\right)^2 \tag{33}$$

Now, to discuss the swelling of glassy polymers, we have to account for the glass transition induced by solvent. Our theory is based on the conventional view that the glass transition a kinetic transition, and we assume that kinetic parameters $\xi$ and $\eta$ change by orders of magnitude at some critical solvent volume fraction $\phi_{\mathrm{cri}}$. We therefore assume that $\xi$ and $\eta$ decrease from glassy value to rubbery value within a range of $2\phi_w$ around $\phi_{\mathrm{cri}}$,

$$\xi(\phi_s) = \xi_r + \frac{1}{2}(\xi_g - \xi_r)\left[1 + \tanh\left(\frac{\phi_{\mathrm{cri}} - \phi_s}{\phi_w}\right)\right] \tag{34}$$

$$\eta(\phi_s) = \eta_r + \frac{1}{2}(\eta_g - \eta_r)\left[1 + \tanh\left(\frac{\phi_{\mathrm{cri}} - \phi_s}{\phi_w}\right)\right] \tag{35}$$

where $\xi_g$ and $\eta_g$ ($\xi_r$ and $\eta_r$) are the material values in the glassy state (and rubbery state), and $\phi_w$ is the width of the glass transition region.

Finally, the energy dissipation for glassy polymers, which includes both $\Phi_{\mathrm{dif}}$ (eq. (28)) and $\Phi_{\mathrm{rhe}}$ (eq. (33)), is written as

$$\frac{\Phi}{L_0^2} = \int_{-h_0}^{h_0} \mathrm{d}z\left[\frac{1}{2}\xi(\phi_s)\left(\dot{u} + 2\dot{\alpha}z\right)^2 + \frac{2}{3}\eta(\phi_s)\left(\frac{\partial \dot{u}}{\partial z} - \dot{\alpha}\right)^2\right] \tag{36}$$

### C. Evolution Equations

The Rayleighian of swelling glassy polymer is given by $\Re = \Phi_{\mathrm{dif}} + \Phi_{\mathrm{rhe}} + \dot{F}$. For the convenience of derivation, we define a variable $w(z,t) = u(z,t) + 2\alpha(t)z$ and replace $u(z,t)$

by $w(z,t)$. The set of state variables then becomes $w(z,t)$ and $\alpha(t)$. Due to the symmetry with respect to the $z=0$ plane, we only consider the polymer in $z \in [0, h_0]$. The free energy eq. (24), the diffusion dissipation eq. (28) and the viscosity dissipation eq. (33) become

$$\frac{F}{L_0^2} = \int_0^{h_0} \mathrm{d}z \left[\frac{1}{2} K \left(w' - 3\varepsilon_{\mathrm{eq}}\right)^2 + \frac{2}{3} G \left(w' - 3\alpha\right)^2\right] \tag{37}$$

$$\frac{\Phi_{\mathrm{dif}}}{L_0^2} = \int_0^{h_0} \mathrm{d}z \frac{1}{2} \xi\left(w'\right) \dot{w}^2 \tag{38}$$

$$\frac{\Phi_{\mathrm{rhe}}}{L_0^2} = \int_0^{h_0} \mathrm{d}z \frac{2}{3} \eta\left(w'\right) \left(\dot{w}' - 3\dot{\alpha}\right)^2 \tag{39}$$

where $w' = u' + 2\alpha = \phi_s$ according to eq. (9). The Rayleighian function then becomes

$$\begin{aligned}\frac{\Re}{L_0^2} = \int_0^{h_0} \mathrm{d}z \; &\left[K \left(w' - 3\varepsilon_{\mathrm{eq}}\right) \dot{w}' + \frac{4}{3} G \left(w' - 3\alpha\right)\left(\dot{w}' - 3\dot{\alpha}\right)\right. \\ &\left. + \frac{1}{2} \xi\left(w'\right) \dot{w}^2 + \frac{2}{3} \eta\left(w'\right)\left(\dot{w}' - 3\dot{\alpha}\right)^2\right] \end{aligned} \tag{40}$$

The minimum condition of $\delta\Re/\delta\dot{w} = 0$ ($\frac{\partial}{\partial z}\frac{\partial R}{\partial \dot{w}'} - \frac{\partial R}{\partial \dot{w}} = 0$ and $\frac{\partial R}{\partial \dot{w}'}\Big|_{z=h_0} = 0$, $R$ is the density of Rayleighian function) and $\delta\Re/\delta\dot{\alpha} = 0$ gives time evolution equations and boundary condition. The time evolution equations are

$$\xi(w')\dot{w} = (K + \frac{4}{3}G) w'' + \frac{4}{3}\frac{\partial}{\partial z}\left[\eta(w')\left(\dot{w}' - 3\dot{\alpha}\right)\right] \tag{41}$$

$$G\left(w - 3\alpha h_0\right) + \int_0^{h_0} \eta(w')\left(\dot{w}' - 3\dot{\alpha}\right)\mathrm{d}z = 0 \tag{42}$$

or written in state variables $u(z,t)$ and $\alpha(t)$,

$$\xi(\phi_s)(\dot{u} + 2\dot{\alpha}z) = (K + \frac{4}{3}G) u'' + \frac{4}{3}\frac{\partial}{\partial z}\left[\eta(\phi_s)\left(\dot{u}' - \dot{\alpha}\right)\right] \tag{43}$$

$$G\left(u - \alpha h_0\right) + \int_0^{h_0} \eta(\phi_s)\left(\dot{u}' - \dot{\alpha}\right)\mathrm{d}z = 0 \tag{44}$$

and at the boundary $z = h_0$,

$$\frac{4}{3}\eta\left(\dot{\phi}_s - 3\dot{\alpha}\right) + K\left(\phi_s - 3\varepsilon_{\mathrm{eq}}\right) + \frac{4}{3}G\left(\phi_s - 3\alpha\right) = 0 \tag{45}$$

where $\phi_s = u' + 2\alpha$ is the solvent volume fraction. The boundary condition at $z=0$ is

$$u = 0 \tag{46}$$

Equations (43)-(46) are the set of equations that determine the time evolution of the sample during swelling.

## D. Induction Time

The induction time $t_{\mathrm{ind}}$ can be analytically solved by the boundary condition eq. (45). In the induction period, we have $\eta = \eta_g$, $\dot{\alpha} = 0$ and $\alpha = \phi_0/3$ since the polymer network is in glassy state. Therefore eq. (45) becomes an ODE for $\phi_s$,

$$\frac{4}{3}\eta_g \dot{\phi}_s + K\left(\phi_s - 3\varepsilon_{\mathrm{eq}}\right) + \frac{4}{3}G\left(\phi_s - \phi_0\right) = 0 \tag{47}$$

It gives analytical solution,

$$\phi_s = \frac{4G\phi_0 + 3K\phi_{\mathrm{eq}}}{4G + 3K} - \frac{3K}{4G + 3K}\left(\phi_{\mathrm{eq}} - \phi_0\right)\exp\left[-\frac{4G + 3K}{4\eta_g}t\right] \tag{48}$$

where $\phi_0$ is the initial solvent volume fraction, $\phi_{\mathrm{eq}} = 3\varepsilon_{\mathrm{eq}}$ is the equilibrium solvent volume fraction. The induction time $t_{\mathrm{ind}}$ is the time at which $\phi_s$ reaches $\phi_{\mathrm{cri}}$. Using equation (48),

$$t_{\mathrm{ind}} = -\frac{4\eta_g}{4G + 3K}\ln\left[1 - \frac{(4G + 3K)(\phi_{\mathrm{cri}} - \phi_0)}{3K(\phi_{\mathrm{eq}} - \phi_0)}\right] \tag{49}$$

We will take $\phi_{\mathrm{cri}} = 0.02$, $\phi_{\mathrm{eq}} = 0.3$ and $\phi_0 < \phi_{\mathrm{cri}}$ in the following. Since both $\phi_0$ and $\phi_{\mathrm{cri}}$ are small values comparing to $\phi_{\mathrm{eq}}$, eq. (49) can be expanded as

$$t_{\mathrm{ind}} \approx \frac{4\eta_g}{3K}\frac{\phi_{\mathrm{cri}} - \phi_0}{\phi_{\mathrm{eq}}} \tag{50}$$

# II. NUMERICAL CALCULATION FOR THE CHARACTERISTIC TIMES

In this section, we explain how we numerically calculate the characteristic times from the full model.

We take $h_0$ as the unit of length and the swelling time in rubbery state, $\tau_{\mathrm{dif}} = h_0^2/D_r$, as the unit of time, where $D_r = (K + \frac{4}{3}G)/\xi_r$ is the diffusivity of solvent in rubbery polymers. For all calculations, we set the equilibrium strain $\varepsilon_{\mathrm{eq}} = 0.1$ (thus $\phi_{\mathrm{eq}} = 0.3$), the solvent volume fraction at glass transition $\phi_{\mathrm{cri}} = 0.02$, and the elastic constant ratio $G/K = 0.1$. We set the transition width $\phi_w = 0.001$ so that the transition region between glassy and rubbery state is negligible. Then, the swelling of glassy polymers is determined by three material parameters, the friction coefficient in glassy state $\xi_g$, the internal viscosity in glassy state $\eta_g$ and in rubbery state $\eta_r$.

Figure S1(a) is a typical snapshot of solvent profile in the swelling process. We can obtain the front position from such a profile. We take the position at which $\phi_s = \phi_{\mathrm{cri}}$ as the Case II

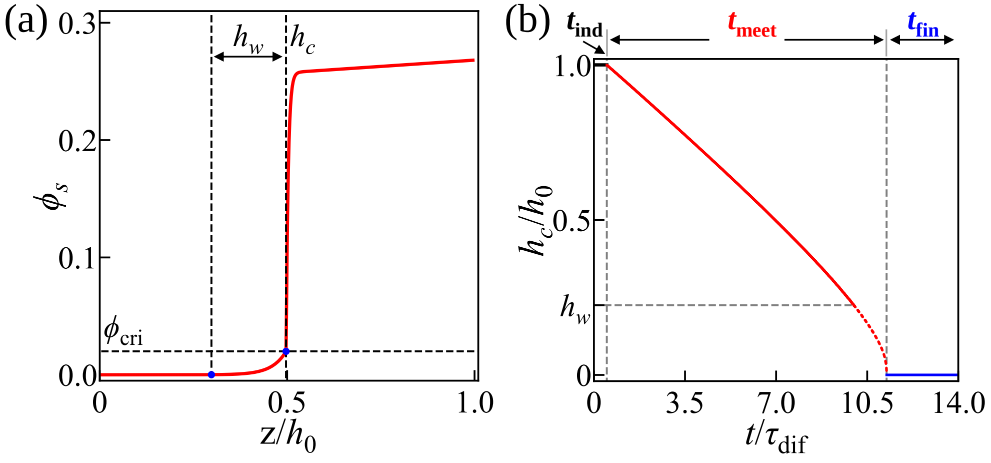


FIG. S1. (a) Typical snapshot of solvent profile of Case II diffusion. The horizontal dashed line indicates the critical solvent volume fraction $\phi_{\rm cri}$. The vertical dashed line in the right is the position where $\phi_s = \phi_{\rm cri}$, corresponding to the front position $h_c$. The left dashed line is the position where $\phi_s = 0.0001$, the region between the two vertical dashed lines is the Fickian precursor, $h_w$. (b) Time evolution of the front position $h_c/h_0$. The duration time of the black part is $t_{\rm ind}$, of the red part is $t_{\rm meet}$, and it of the blue part is $t_{\rm fin}$. The red dashed line is the time evolution of $h_c$ after the two precursor touch each other. This figure is calculated under $\xi_g/\xi_r = 5000$, $\eta_g/\eta_r = 100$, and $\eta_r/\xi_r h_0^2 = 0.05$.

front position (the vertical dashed line in the right with label $h_c$). Then, the entire $h_c(t)$ of the swelling process can be obtained from the time evolution of solvent profile. Figure S1(b) shows one case of the time evolution of $h_c(t)$. Once we have the front position, the three characteristic times, $t_{\rm ind}$, $t_{\rm meet}$ and $t_{\rm fin}$, can be calculated from $h_c(t)$, as shown in figure S1(b).

**The calculation of $h_w$:** From the time evolution of solvent profile, we can numerically calculate the Fickian precursor length ahead of the front $h_w(t)$. We record the distance between $h_c(t)$ and the place at which $(\phi_s - \phi_0)/(\phi_{\rm cri} - \phi_0) = 0.005$ as $h_w$ at time $t$. Figure S2(a) is the time evolution of $h_w$ for situations of various solvent initial volume fraction $\phi_0$. It is seen that $h_w$ is nearly flat in case II diffusion stage. Figure S2(b) is the dependence of $\bar{h}_w/h_0$ on $\phi_{\rm cri} - \phi_0$. Here, $\bar{h}_w$ is the time averaged value of $h_w$ over the case II diffusion stage corresponding to a given $\phi_0$. Results show that $\bar{h}_w$ nearly remains unchanged when $\phi_{\rm cri} - \phi_0$ changes from 0 to 0.02, while all other parameters are fixed. Results in Fig. S2 indicate that $h_w$ is independent of $\phi_0$, and is a material determined parameter.

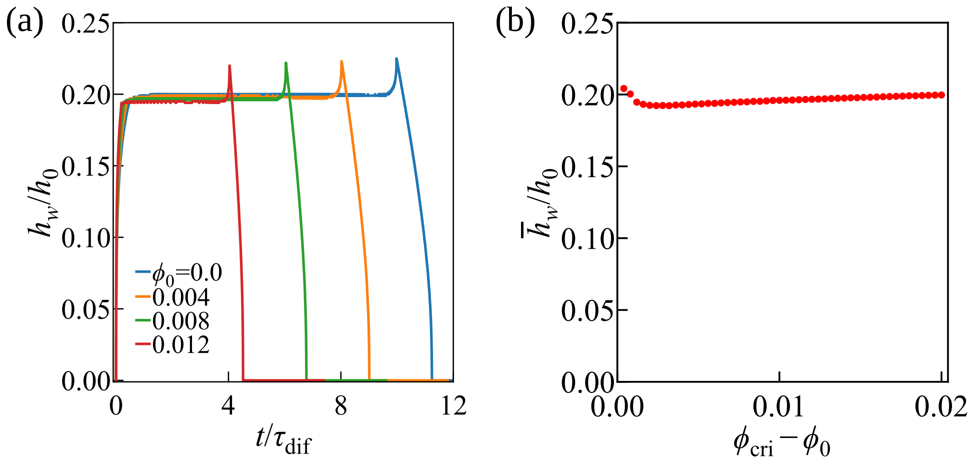


FIG. S2. (a) Time evolution of the Fickian precursor length $h_w/h_0$ for four values of the initial solvent volume fraction $\phi_0$. The time is scaled by the diffusion time $\tau_{\text{dif}}$. (b) The dependence of time averaged Fickian precursor length $\bar{h}_w$ on $\phi_{\text{cri}} - \phi_0$. All other parameters for these calculations are $\xi_g/\xi_r = 5000$, $\eta_g/\eta_r = 100$ and $\eta_r/\xi_r h_0^2 = 0.05$.

**The calculation of $t_{\text{ind}}$:** The black part in figure S1(b) is the induction period. We numerically record the time at which the solvent volume fraction at the surface reaches $\phi_s|_{z=h_0} = \phi_{\text{cri}} = 0.02$ as $t_{\text{ind}}$.

As there are three independent parameters in the model, the calculation of $t_{\text{ind}}$ for a given $\eta_g/K$ is not unique. This is because that for a given $\eta_g$, the full model can be solved under different values of $\eta_r$ and $\xi_g$. Figure S3(a) illustrates this issue, where different color stands for different value of $\eta_g$, and different shape of label represents for different value of $\eta_r$. Results show that as long as $\eta_g$ is fixed, $t_{\text{ind}}$ remains nearly unchanged for different set values of $\eta_r$ and $\xi_g$. In other words, $t_{\text{ind}}$ is dominated by $\eta_g$, confirming our analytical results indicated by solid lines.

**The calculation of $t_{\text{meet}}$:** The duration time of the red part in figure S1(b) is $t_{\text{meet}}$. In numerical calculations, we record the duration time of the solvent volume fraction at the middle plane reaching at $\phi_s|_{z=0} = \phi_{\text{cri}} = 0.02$ after the induction period as the $t_{\text{meet}}$.

**The calculation of $t_{\text{fin}}$:** The duration time of the last relaxation stage is $t_{\text{fin}}$, corresponding to the blue part in figure S1(b). We record the duration time of the solvent volume fraction at the middle plane changing from $\phi_s|_{z=0} = \phi_{\text{cri}}$ to $\phi_s|_{z=0} = 0.999\phi_{\text{eq}}$ as $t_{\text{fin}}$.

**The calculation of $v_{\text{front}}$:** In numerical calculation, $v_{\text{front}}$ is obtained by calculating

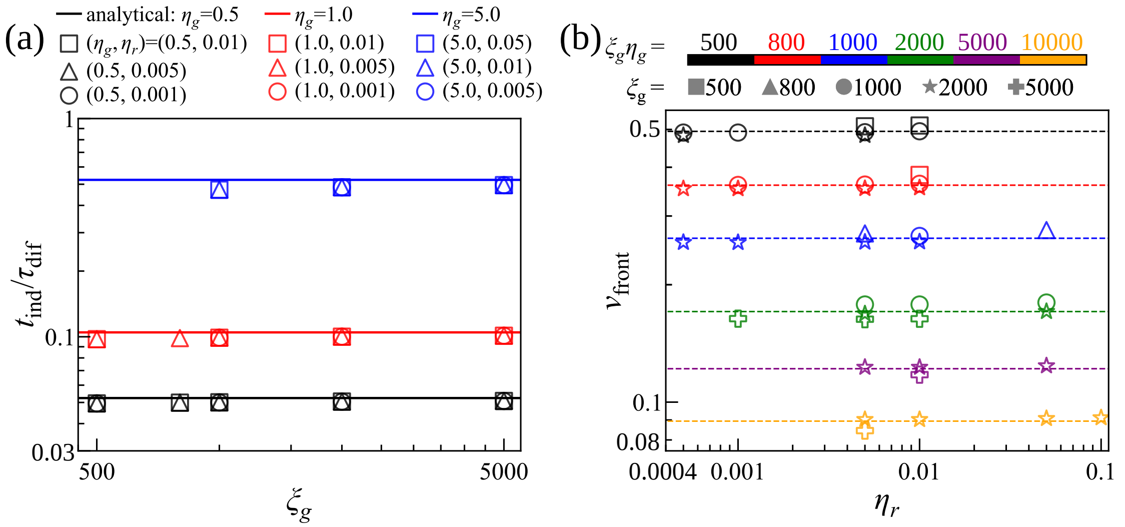


FIG. S3. (a) The dependence of induction time $t_{\mathrm{ind}}/\tau_{\mathrm{dif}}$ on $\xi_g$. All data points are numerically calculated from the full model, while all solid lines are analytical results of Eq. (50). The color stands for the value of $\eta_g$, while the shape of label represents for the value of $\eta_r$. Different set values of $(\eta_g, \eta_r)$ used for our calculations are listed on the top of figure. (b) The dependence of front velocity $v_{\mathrm{front}}$ on $\eta_r$, where $v_{\mathrm{front}}$ is in the units of $h_0/\tau_{\mathrm{dif}}$. All data points are numerical results from the full model, while all dashed lines are the average value of $v_{\mathrm{front}}$ for given $\eta_g\xi_g$. The color stands for the value of $\eta_g\xi_g$, while the shape of label represents for the value of $\xi_g$.

the slope of the red solid part of the time evolution of $h_c(t)$ shown in figure S1(b). We record the front position $h^*$ for a time when the solvent volume fraction at the middle plane reaches at $\phi_s|_{z=0} = 0.0001$ (for non-zero $\phi_0$, we record the front position $h^*$ when $(\phi_s|_{z=0} - \phi_0)/(\phi_{\mathrm{cri}} - \phi_0) = 0.005$). In fact, $h^*$ is the precursor length $h_w$ according to our definition in figure S1(a). Then, the slope $(h_0 - h_w)/t_{\mathrm{meet}}$ is the $v_{\mathrm{front}}$.

The calculation of the front velocity $v_{\mathrm{front}}$ has the same feature as the calculation of $t_{\mathrm{ind}}$. The value of $\sqrt{D_g K/\eta_g}$ is related to the combined parameter $\eta_g\xi_g$. Therefore, the calculation of the dependence of $v_{\mathrm{front}}$ on $\sqrt{D_g K/\eta_g}$ is not unique neither because we have different combinations of $\eta_g$ and $\xi_g$ for a given $\sqrt{D_g K/\eta_g}$. Figure S3(b) shows that $v_{\mathrm{front}}$ remains the same as long as the value of $\eta_g\xi_g$ is fixed, indicating that $v_{\mathrm{front}}$ is not dependent on the individual value of $\eta_g$ and $\xi_g$. In figure S3(b), the color stands for the value of $\eta_g\xi_g$, while the shape of label represents for the value of $\xi_g$.

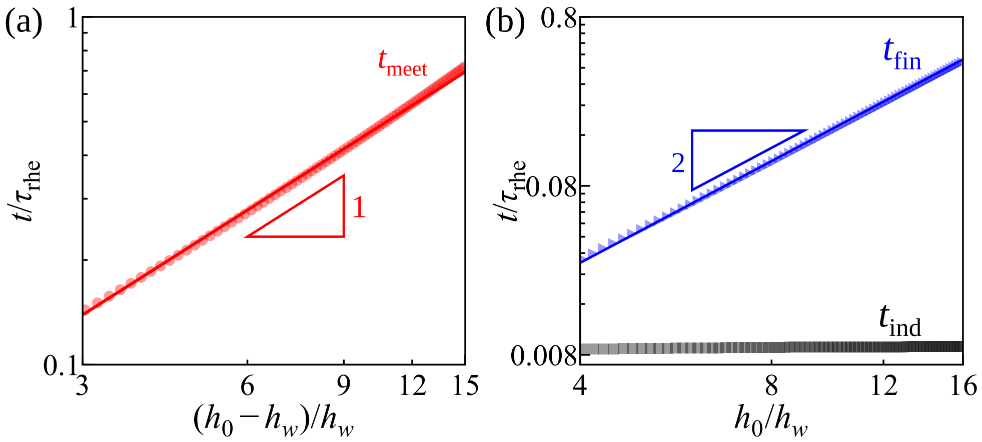


FIG. S4. (a) The dependence of $t_{\mathrm{meet}}/\tau_{\mathrm{rhe}}$ on $(h_0 - h_w)/h_w$. (b) The dependence of $t_{\mathrm{ind}}/\tau_{\mathrm{rhe}}$ and $t_{\mathrm{fin}}/\tau_{\mathrm{rhe}}$ on $h_0/h_w$. Data points are numerically results for $\xi_g/\xi_r = 5000$, $\eta_g/\eta_r = 100$, and $h_0/h_w \in [4, 16]$. All solid lines are guiding lines.

## III. DEPENDENCE OF THE CHARACTERISTIC TIMES ON INITIAL THICKNESS

We also numerically checked the dependence of the characteristic times on the initial thickness $h_0$. Figure S4(a) is the log-log plot of the effects of $h_0 - h_w$ on the Case II diffusion time. Since $h_0$ is not a constant, we now use $h_w$ as the new length unit and use $\tau_{\mathrm{rhe}} = \eta_g/G$ as the new timescale. In this set of units, the independent parameters become $\eta_g/\eta_r$, $\xi_g/\xi_r$ and $h_0/h_w$. The red data points are $t_{\mathrm{meet}}$ calculated from the full model for various $h_0$, while the red solid line is the guide linear line with a slope of 1. Results show that $t_{\mathrm{meet}} \sim h_0 - h_w$. Figure S4(b) is the similar comparison between the result of full numerical calculation and the result of scaling analysis for induction time, $t_{\mathrm{ind}}$, and Fickian expansion time $t_{\mathrm{fin}}$. The blue data points are calculated $t_{\mathrm{fin}}$, which show that $t_{\mathrm{fin}}$ is proportional to $h_0$ to the power of 2, i.e., $t_{\mathrm{fin}} \sim h_0^2$. The black data points show that $t_{\mathrm{ind}}$ is independent on $h_0$. All numerical results are consistent with the analytical scaling laws.

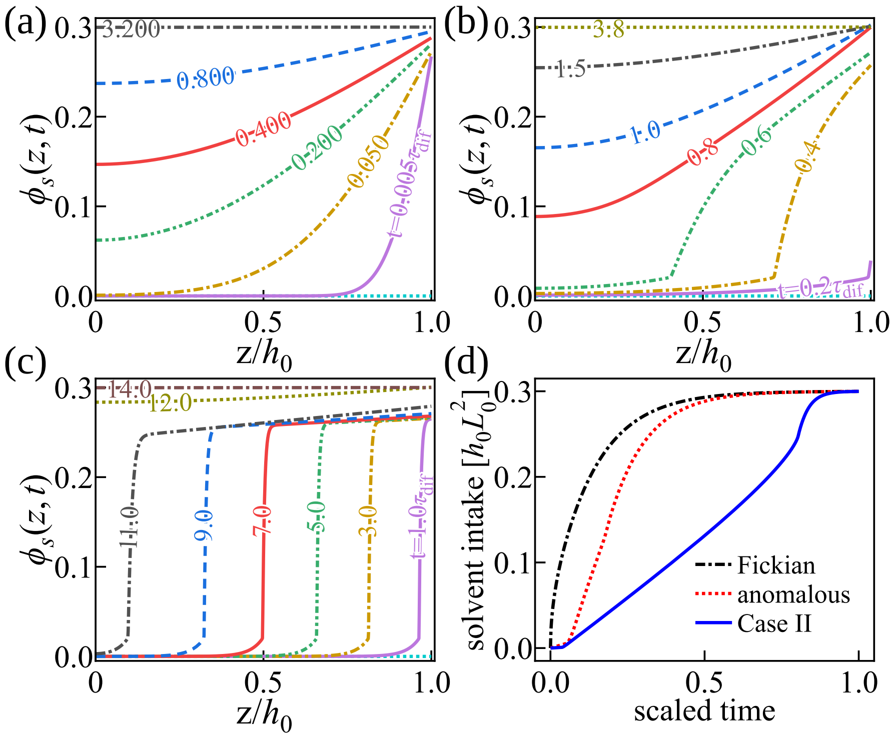


FIG. S5. Different diffusion behaviors ranging from (a) Fickian, (b) anomalous, and (c) Case II. The solvent intake of the three process is plotted in (d). The time in (d) is scaled by the time at which the whole polymer is fully swollen by solvent, defined by the last instant of $t_{\rm fin}$ (See Figure S1). The calculation parameters are (a) $\xi_g/\xi_r = 1$, and $\eta_g = \eta_r = 0$, (b) $\xi_g/\xi_r = 50$, $\eta_g = \eta_r = 50$ and $\eta_r/\xi_r h_0^2 = 0.05$, (c) $\xi_g/\xi_r = 5000$, $\eta_g = \eta_r = 100$ and $\eta_r/\xi_r h_0^2 = 0.05$, other parameters are the same as the manuscript.

## IV. THE VALIDITY OF THE MODEL

### A. Our model predicts a broader range of diffusion behaviors from Fickian to super Case II diffusion.

Figure S5(a) shows a Fickian diffusion behavior. This result is obtained by solving eqn. (3)-(4) of the manuscript for the parameter set $\xi_g/\xi_r = 1$, and $\eta_g = \eta_r = 0$. This corresponds to the usual swelling of soft polymers, in which the dissipation energy due to viscosity is negligible. Figure S5(b) shows anomalous diffusion behavior obtained by setting $\xi_g/\xi_r = 50$, $\eta_g/\eta_r = 50$ and $\eta_r/\xi_r h_0^2 = 0.05$. Figure S5(c) is the Case II diffusion behavior for the same

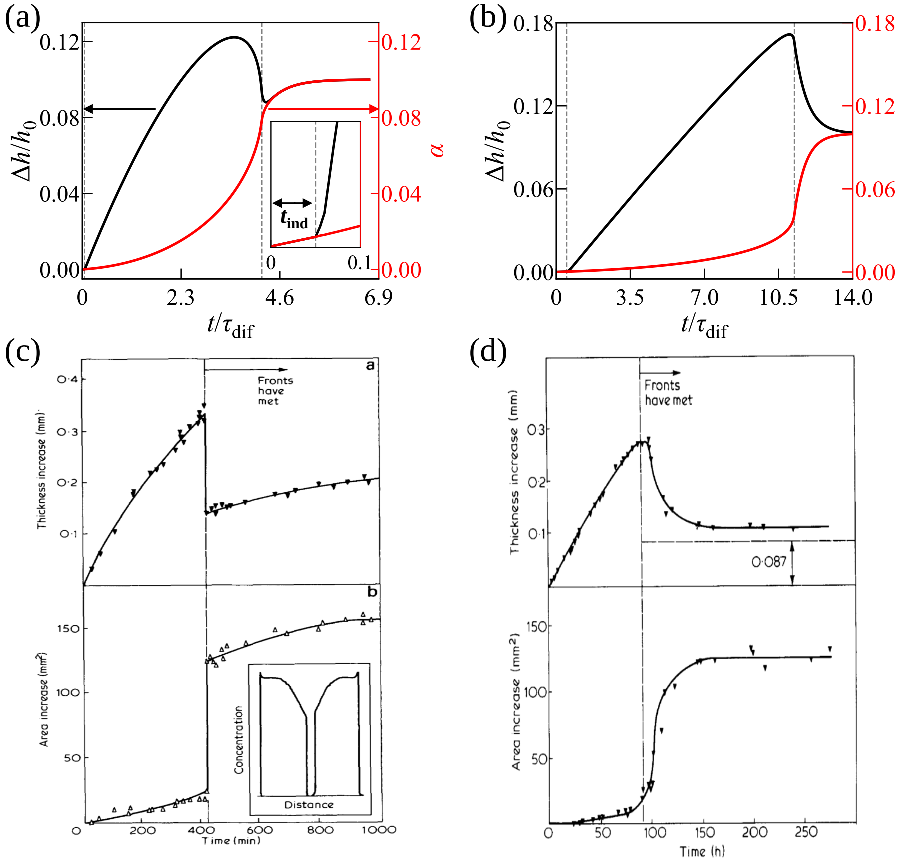


FIG. S6. Comparison between calculated shape evolution (a) (b) and experimental results (c) (d) of PMMA-methanol sample by Thomas and Windle [9]. In (a) and (b), black solid line is the time dependence of the strain normal to the surface and red solid line is the strain parallel to the surface. In (c) and (d), the upper plot is strain normal to the surface and the lower panel is the strain parallel to the surface. (a) is the calculated shape evolution with lower viscosity ($\eta_r/\xi_r h_0^2 = 0.005$), which shows similar trend as the experiment result (c) at high temperature (42°C). (b) is the calculated shape evolution with higher viscosity ($\eta_r/\xi_r h_0^2 = 0.05$), corresponding to experiment result (d) at low temperature (24°C).

parameter set as in Fig. 2(a) of the manuscript. For these three cases, we also calculated solvent intake, $u(h_0, t) + 2\alpha(t)$ and showed it in Figure S5(d). In the case of Fickian diffusion (dashed-black line), the solvent intake is proportional to the square root of time t. In the case of anomalous diffusion (dotted-red line), the solvent intake is proportional to $t^a$ with the exponent $a$ between 0.5 and 1. In the Case II diffusion (solid-blue line), the solvent intake

increases linearly in time, and suddenly accelerates when the solvent fronts meet, aligning with the characteristics of super Case II diffusion behavior.

### B. Our model explains the two types of the relaxation behavior observed by Thomas and Windle in the second stage.

Thomas and Windle observed that in the swelling of PMMA at 42°C, the thickness first decreases and increases again towards the equilibrium value, as shown Figure S6(c). On the other hand, in the swelling at 24°C, the thickness decreases monotonically to the equilibrium value as shown Figure S6(d). We conducted the calculation for two cases, $\eta_r/\xi_r h_0^2 = 0.005$, and $\eta_r/\xi_r h_0^2 = 0.05$. The former corresponds to high viscosity and corresponds to the swelling at low temperature, and the latter corresponds to the swelling at high temperature. Our results are in agreement with experimental results and indicates the importance of rheological properties on the swelling.

---


[1] Masao Doi. Gel dynamics. *Journal of the Physical Society of Japan*, 78(5):052001, 2009.

[2] Masao Doi. *Soft matter physics*, pages 116,174. Oxford University Press, 2013.

[3] Masao Doi. Onsager principle in polymer dynamics. *Prog. Polym. Sci.*, 112:101339, 2021.

[4] Lev Davidovich Landau, Evgenii Mikhailovich Lifshitz, Arnol'd Markovich Kosevich, and Lev Petrovich Pitaevskii. *Theory of elasticity*, page 15. Elsevier, 1986.

[5] Xingkun Man and Masao Doi. Swelling dynamics of a disk-shaped gel. *Macromolecules*, 2021.

[6] Zhaoyu Ding, Peihan Lyu, Ang Shi, Xingkun Man, and Masao Doi. Diffusio-mechanical theory of gel bending induced by liquid penetration. *Macromolecules*, 2022.

[7] Peihan Lyu, Zhaoyu Ding, and Xingkun Man. Accelerating the stimuli-responsive bending of a gel using mechanical constraints. *The European Physical Journal E*, 46(6):40, 2023.

[8] Jean Lemaitre. Section 2.1 - introduction to elasticity and viscoelasticity. In Jean Lemaitre, editor, *Handbook of Materials Behavior Models*, pages 71–74. Academic Press, Burlington, 2001.

[9] Noreen Thomas and A. H. Windle Discontinuous shape changes associated with Case II transport of methanol in thin sheets of PMMA *Polymer*, 18:1195, 1977.
